# Supplementary material for: Free electron emission in vacuum assisted by photonic time crystals
Source: arXiv:2311.01203 source file (2023-11-02)
Supplement: Supplementary file 1 [file Supplementary.pdf]

# Supplementary material: Free electron emission in vacuum assisted by photonic time crystals

Xiaoke Gao, Xiaoyu Zhao, Xikui Ma, Tianyu Dong *
School of Electrical Engineering, Xi'an Jiaotong University, Xi'an 710049, China
*To whom correspondence should be addressed; E-mail: tydong@mail.xjtu.edu.cn.

## S1 Comparison between traditional Smith–Purcell effects and temporal Smith–Purcell radiation

Smith–Purcell (SP) radiation is produced when an electron traverses in close proximity over a periodic surface (grating), causing charges on the surface of the grating to rearrange in order to obstruct the electron's path, thereby resulting in the emission of electromagnetic radiation. It is determined that the radiated wavelength $\lambda$ is dependent on the pitch of the grating $d$ and the velocity of the electron $\beta = v/c_0$, where $c_0$ is the speed of light in vacuum, which reads

$$\lambda = \frac{d}{n}\left(\frac{1}{\beta} - \cos\theta\right), \tag{S1}$$

where $n$ denotes the diffraction order and $\theta$ signifies the angle of emission as measured in the direction of beam propagation. In the context of a single electron beam, Smith–Purcell radiation manifests in all directions in the vacuum (*1*,*2*), implying the difficulty in distinguishing particles. Pre-bunched beams that are repeated periodically during the bunching process have been used to obtain monochromatic and directional radiation with enhanced intensity. In practice, the beam bunching frequency $\omega_b$ corresponds to the frequency at which the dispersion relation for the grating intersects with the beam line (*3*), as shown in Fig. S1A. The aforementioned enhanced radiation is also referred to as super-radiance or coherent Smith–Purcell (CSP) radiation (*4*, *5*), which is characterized by the relation between the radiated wavelength $\lambda$ and the particle velocity $\beta$, as indicated in (S1). Super-radiance or CSP radiation has been demonstrated both in theoretical analysis (*1*) and experimental investigations (*6*), showing an improvement of the radiation at the bunching frequency and its harmonics.

When fast particles move in close proximity over a temporally modulated medium, such as PTCs, radiations can also be observed in the free space, resembling the traditional SP radiation. Unlike conventional SP radiation, the radiated wavelength $\lambda$ depends on the modulation

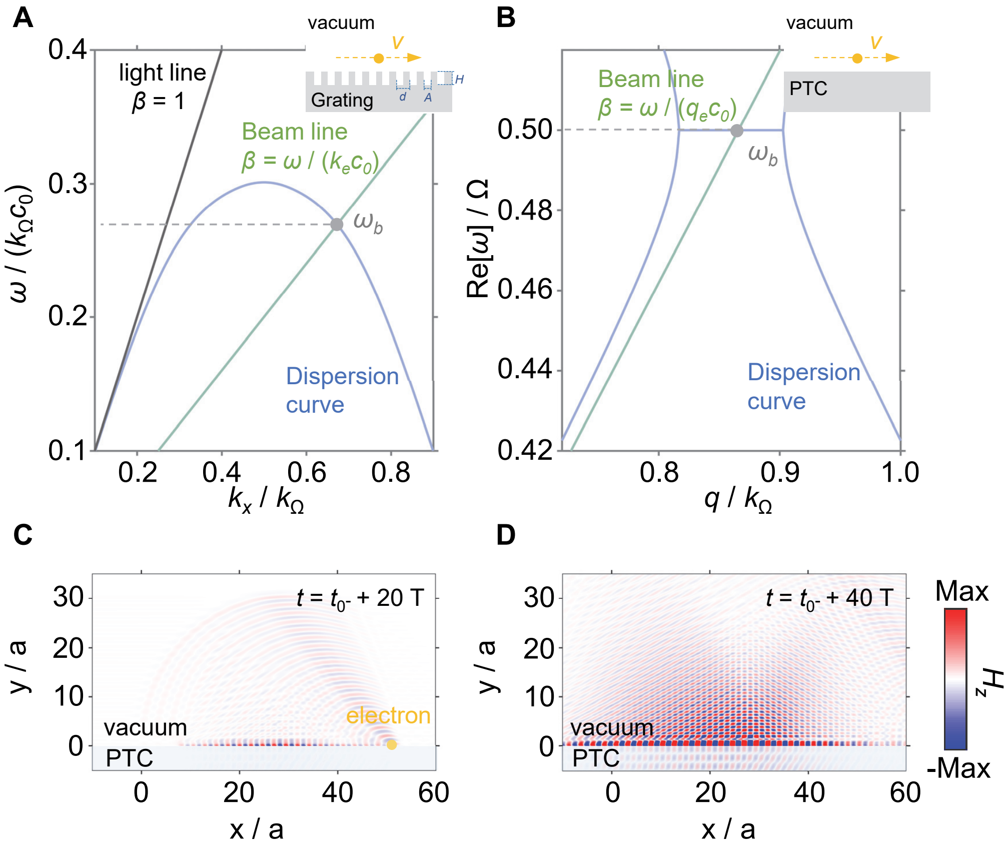


Figure S1: **Comparison between traditional Smith–Purcell effects and temporal Smith–Purcell radiation.** (**A**) Dispersion relation of the surface waves of the grating made of perfect conductor, whose parameters are: groove width $A = 62$ μm, groove depth $H = 100$ μm and period $d = 173$ μm as given in (*5*). The dispersion curves of the grating are shown in blue; as references, the black line represents the light line in vacuum and the green line represents the beam line. (**B**) The dispersion relation for the waves in the PTC. The blue line and the green line represent the dispersion curve for waves and the beam line in PTC, respectively. Note that the light line $\beta = 1$ is absent because it is outside the plot range. The permittivity of the PTC is $\varepsilon(t) = \varepsilon_r(1 + \alpha \sin \Omega t)$ with $\varepsilon_r = 3$ and $\alpha = 0.2$, which is the same as for **Figure 2** in the main text. (**C** and **D**) Near-field magnetic field distribution $H_z$ when $t = t_{0^-} + 20T$ and $t = t_{0^-} + 40T$, respectively, where $t_{0^-}$ denotes the modulation starting time and $T = 2\pi/\Omega$ denotes the modulation period.

frequency $\Omega$, the velocity of the particles $\beta$, and the radiation angle $\theta$, which reads

$$\lambda = \frac{d'_\Omega}{n}\left(\frac{1}{\beta} - \cos\theta\right), \tag{S2}$$

where $d'_\Omega = 2\pi/\Omega \cdot c_0/\cos\theta$ and $n$ denotes the harmonic order. Interestingly, the relation (S2)

is quite similar to (S1) for traditional SP radiation; thus, we would refer to such an effect as temporal Smith–Purcell radiation. Fig. S1C depicts the near-field magnetic field $H_z$ around the moving electron in close proximity over a PTC when $t = t_{0^-} + 20T$, where $t_{0^-}$ denotes the start time of the modulation and $T = 2\pi/\Omega$ denotes the modulation period. It can be observed that waves radiate in all directions in vacuum, which is similar to the field distribution for traditional SP radiation (*7, 8*). Furthermore, electron traversing in close proximity over a PTC would result in highly directional radiation emission with high intensity, as shown in Fig. S1D (see also **Figure 2** and **Figure 3** in the main text), which is absent in traditional CSP radiation for single electron beam excitation. Here, the radiation angles $\theta_n$ and frequencies $\omega = \omega_b + n\Omega$ obey (S2), where the fundamental frequency $\omega_b$ of the radiated waves corresponds to the point at which the PTC dispersion curve intersects the beam line, as illustrated in Fig. S1B. Unlike the requirement of periodically repeated electron bunches for CSP radiation, the interaction between a single electron bunch and the PTC can excite pronounced directional propagating waves. This is due to the time-reversal characteristics of the time-varying medium, which supports the generation of the enhanced backward waves with the fundamental frequency of $\omega_b = \Omega/2$ (inter-band mode in MBG), namely time-reversal (TR) waves in the main text, propagating to the vacuum–PTC interface and transmitting into free space to radiate. Therefore, the utilization of PTCs enables the identification of a single particle bunch, which is challenging with conventional SP radiation methods.

# S2 Eigenmode analysis and parametric study on band structures of PTCs

In a nonmagnetic homogeneous material that varies in time, the source-free governing wave equation for electric fields $\mathbf{E}(\mathbf{r},t)$ reads

$$\nabla^2\mathbf{E}(\mathbf{r},t) - \mu_0\partial_t^2[\varepsilon(t)\mathbf{E}(\mathbf{r},t)] = 0. \tag{S3}$$

When the permittivity of the time-varying medium is periodically modulated as $\varepsilon(t) = \varepsilon(t+T)$ with period $T$, it can be expressed in terms of Fourier series as

$$\varepsilon(t) = \sum_{m=-\infty}^{\infty} \varepsilon_m e^{-\mathrm{i}m\Omega t}, \tag{S4}$$

where $\Omega = 2\pi/T$. Consequently, the electric field can be expressed as

$$\mathbf{E}(\mathbf{r},t) = \sum_{n=-\infty}^{\infty} \mathbf{E}_n e^{\mathrm{i}[\mathbf{q}\cdot\mathbf{r} - (\omega + n\Omega)t]} \tag{S5}$$

according to the Floquet theorem, where $\omega$ and $\mathbf{q}$ denote the Floquet quasi-frequency and wave vector, respectively. Inserting the Fourier series (S4) and (S5) into (S3), we can obtain

$$\mu_0(\omega + n\Omega)^2 \sum_{m=-\infty}^{\infty} \varepsilon_{n-m}\mathbf{E}_m = q^2\mathbf{E}_n, \qquad n \in \mathbb{Z}. \tag{S6}$$

In general, the mode numbers $m$ and $n$ are often truncated to a finite maximum mode number $N$ so that the eigenproblem (S6) of infinite dimension can be handled. Within the mode truncation, the eigenproblem (S6) can be rewritten in matrix form as

$$\left[(\mathscr{D}\cdot\mathscr{E})\otimes\mathbb{I}_3 - q^2\mathbb{I}_{2N+1}\right]\cdot\mathbf{\Phi} = 0, \tag{S7}$$

where $\mathbf{\Phi} = [\mathbf{E}_{-N},\ldots,\mathbf{E}_N]^{\mathrm{T}}$. Here, $\mathbb{I}_3$ and $\mathbb{I}_{2N+1}$ denote identity matrices of orders three and $2N+1$, respectively; $\otimes$ denotes the Kronecker product; $\mathscr{D} = \mu_0\mathrm{diag}[(\omega-N\Omega)^2,\ldots,\omega,\ldots,(\omega+N\Omega)^2]$ is a diagonal matrix $\mathscr{E}$ is the matrix that reflects the information of the medium, which reads

$$\mathscr{E} = \begin{pmatrix} \varepsilon_0 & \varepsilon_{-1} & \ldots & \varepsilon_{-2N} \\ \varepsilon_1 & \varepsilon_0 & \ldots & \varepsilon_{-2N+1} \\ \vdots & \vdots & \ddots & \vdots \\ \varepsilon_{2N} & \varepsilon_{2N-1} & \ldots & \varepsilon_0 \end{pmatrix}. \tag{S8}$$

As a result, the band structure (dispersion relation) of the PTC can be obtained by solving

$$\det\left[(\mathscr{D}\cdot\mathscr{E})\otimes\mathbb{I}_3 - q^2\mathbb{I}_{2N+1}\right] = 0. \tag{S9}$$

Furthermore, the $l$-th eigenvector $\phi_l = [\mathbf{E}_{-N,l},\ldots,\mathbf{E}_{N,l}]^{\mathrm{T}}$ corresponds to the $l$-th eigenmode with the $l$-th eigenvalue $q_l^2$ being the wave number. Finally, the electric field can be expressed in terms of $\mathbf{E}_{n,l}$ as

$$\mathbf{E}(\mathbf{r},t) = \sum_{n=-\infty}^{\infty}\sum_{l=1}^{2N+1}\mathbf{E}_{n,l}e^{\mathrm{i}[\mathbf{q}_l\cdot\mathbf{r}-(\omega+n\Omega)t]}. \tag{S10}$$

The band structure of a time-varying medium is dependent on its permittivity. Fig. S2 illustrates the parametric study of static permittivity $\varepsilon_r$ and modulation depth $\alpha$. Since static permittivity $\varepsilon_r$ determines the group and phase velocity of the wave within the PTC, the dispersion curves become flat as the static permittivity is large. Thus, more than one mode may be amplified when the corresponding frequencies within the momentum band gap (MBG) are below the light line. The width of the MBG can be regulated by changing the modulation depth, as demonstrated by Fig. S2D – Fig. S2F. As the modulation depth $\alpha$ increases, the momentum band gap becomes wider.

The band structure of a PTC varies when the modulation type changes, as shown in Fig. S3. For example, by adding the modulation $\alpha_2\sin 2\Omega t$ of a higher frequency to $\varepsilon(t)/\varepsilon_r = 1+\alpha_1\sin\Omega t$, a new momentum gap can be opened compared to Fig. S2A, as shown in Fig. S3D. When the permittivity $\varepsilon(t)$ can be expanded in terms of multiple harmonics, *e.g.*, for the sawtooth and square-wave modulations (Fig. S3B and Fig. S3C, respectively), multiple MBGs can appear, as shown in Fig. S3E and Fig. S3F. When careful design is employed in PTC modulation, it becomes feasible to manipulate the band structure, thereby allowing for customization of the free-electron radiation pattern.

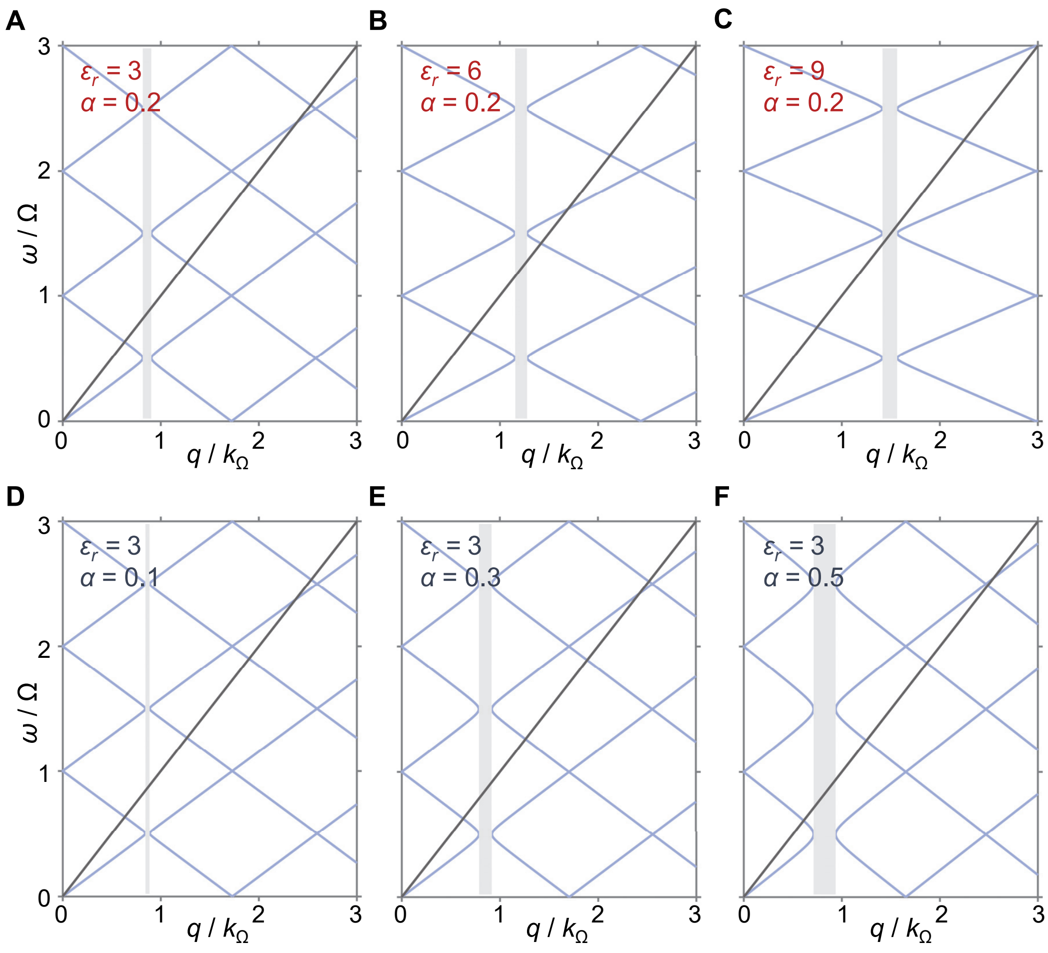


Figure S2: **Parametric study of static permittivity and modulation depth on the band structure of PTCs.** The PTC is sinusoidal modulated as $\varepsilon(t) = \varepsilon_r(1+\alpha\ \sin\Omega t)$. (**A**, **B** and **C**) Band structures of PTC when $\alpha = 0.2$ for various static permittivity, *i.e.*, $\varepsilon_r = 3$, $\varepsilon_r = 6$ and $\varepsilon_r = 9$, respectively. (**D**, **E** and **F**) Band structures of PTC when $\varepsilon_r = 3$ for various modulation depth, *i.e.*, $\alpha = 0.1$, $\alpha = 0.3$ and $\alpha = 0.5$, respectively. The light lines $\omega/q = c_0$ in vacuum are depicted as a reference; and the momentum band gaps are shaded in grey.

# S3 Light emission in various scenarios

## S3.1 When $1 > \beta > \beta_{\text{th}}$

Fig. S4 illustrates the snapshots of the magnetic-field distribution for various time frames. Before the modulation starts, as shown in Fig. S4A, a non-radiative Cerenkov-like electromagnetic field appears inside the PTC region, whereas in vacuum the field is localized around the electron and would not radiate. During PTC modulation, as shown in Fig. S4B and Fig. S4C, TR

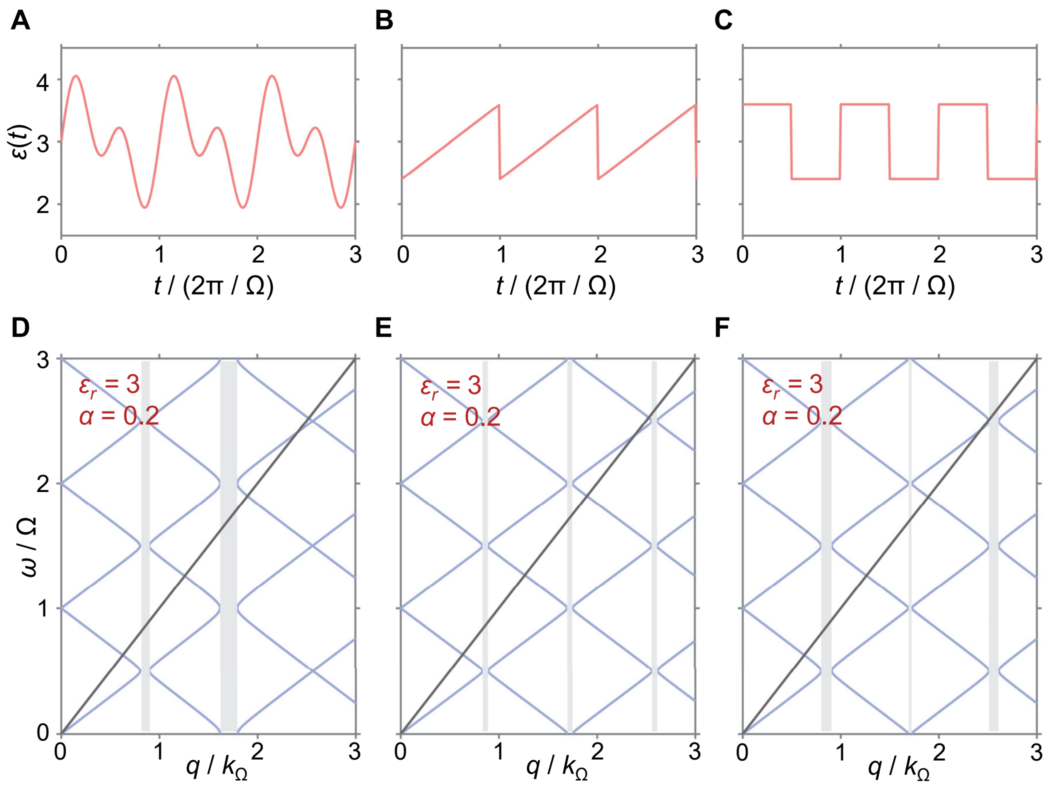


Figure S3: **Band structure of PTCs for various type of modulation.** The modulation functions are $\varepsilon_{\sin}(t) = \varepsilon_r(1+\alpha_1 \sin\Omega t + \alpha_2 \sin 2\Omega t)$, $\varepsilon_{\text{sawTooth}}(t) = \varepsilon_r\{1+2\,\alpha/T\,[t-(1/2+n)\,T]\}$ and $\varepsilon_{\text{pulse}}(t) = \varepsilon_r\{1-\alpha\,\text{sgn}[t-(1/2+n)\,T]\}$ when $n\,T \leq t \leq (n+1)\,T$ and $n \in \mathbb{Z}$. Here, $T = 2\pi/\Omega$, $\varepsilon_r = 3$ and $\alpha_1 = \alpha_2 = \alpha = 0.2$. (**A**, **B** and **C**) Relative permittivity of $\varepsilon_{\sin}(t)$, $\varepsilon_{\text{sawTooth}}(t)$ and $\varepsilon_{\text{pulse}}(t)$, respectively, as functions of time, $t$. (**D**, **E** and **F**) Band structures of PTCs corresponding to **A**, **B** and **C**, respectively. The light lines $\omega/q = c_0$ in vacuum are depicted as a reference; and the momentum band gaps are shaded in gray.

waves exhibit in the PTC and propagate towards the PTC–vacuum interface. As a result, some of the extraordinary waves transmit into the free space as propagating plane waves, and others produce surface waves at the interface due to the total reflection. In addition, the intensity of the propagating and surface waves will increase with the time during the modulation. Unlike conventional Cerenkov radiation that is not monochromatic (*9*) and the Smith–Purcell effect that is not directional (*10*), we emphasize that this PTC-assisted Cerenkov-like radiation is both monochromatic and highly directional, which is useful not only for particle detection, but also for the design of innovative radiation sources. After the modulation is terminated, as shown in Fig. S4D, the existing plane waves would continue to propagate opposite to the interface, and the new propagating plane wave would no longer be produced and transmitted from the interface (PTC); also, the surface waves would gradually attenuate.

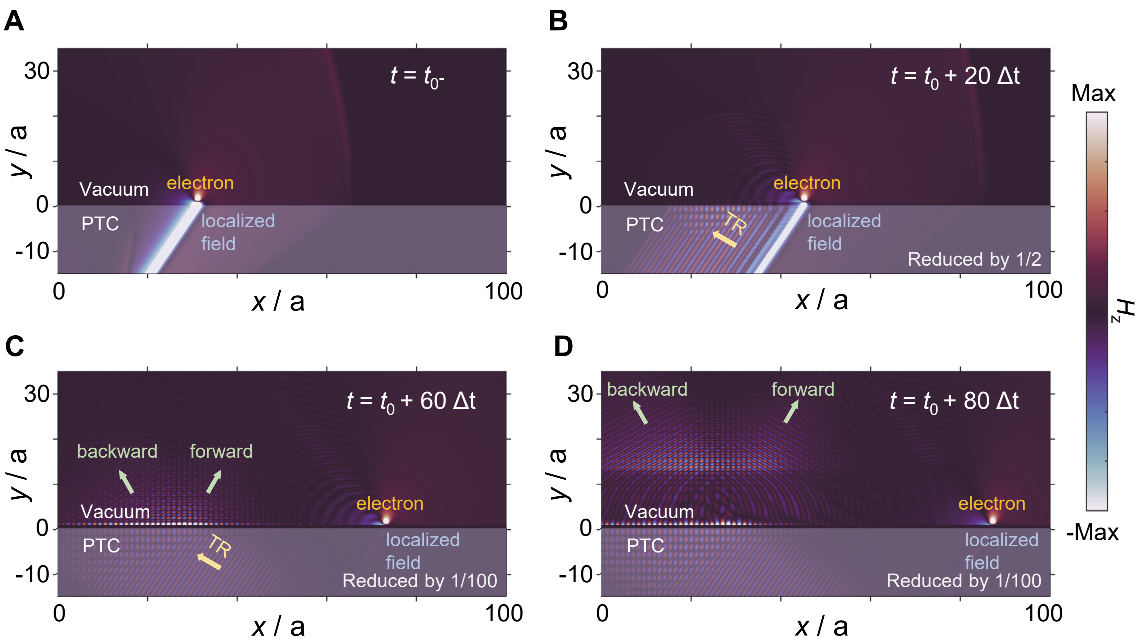


Figure S4: **Snapshots of the magnetic field distribution at various time frame.** They respectively correspond to (**A**) $t = t_{0^-}$ just before the modulation, (**B**) $t = t_0 + 20\Delta t$ and (**C**) $t = t_0 + 60\Delta t$ during the modulation, and (**D**) $t = t_0 + 80\Delta t$ after the modulation stops. The PTC substrate in the $y < 0$ region starts to modulate at $t = t_0$ and lasts for $65\Delta t = 40T_{\text{mod}}$, where $T_{\text{mod}} = 2\pi/\Omega$ is the period of the modulation. The simulation parameters are the same as **Figure 2** in the main text.

## S3.2 When $\beta < \beta_{\text{th}}$

In the main text, it is demonstrated that highly directional monochromatic radiation appears when the particle velocity exceeds the threshold, *i.e.*, $\beta > \beta_{\text{th}}$, which is determined by the static permittivity $\varepsilon_r$ as $\beta_{\text{th}} = 1/\sqrt{\varepsilon_r}$. When the velocity of the particles is smaller than the threshold for low-energy particles, as illustrated in Fig. S5A, the radiation in the vacuum is negligible and no surface waves appear at the vacuum–PTC interface. For example, when $\beta = 0.4 < \beta_{\text{th}} = 1/\sqrt{3} \approx 0.58$, as depicted in the band structure in Fig. S5C, the tangential momentum $k_e$ of the confined mode corresponding to frequency $\omega_{b,0}$ exceeds the MBG of the PTC; consequently, the inter-band mode in the PTC cannot be excited; thus, it does not produce high-intensity radiation in vacuum. Furthermore, since the velocity of particles $\beta$ is below the threshold $\beta_{\text{th}}$, Cerenkov-like radiation with directional propagation no longer exists before PTC modulation. Consequently, when modulation begins, the TR waves would exhibit various propagation directions, leading to the absence of directional propagation waves in vacuum. In comparison, when the static permittivity of the PTC is increased to $\varepsilon_r = 12$ such that $\beta = 0.4 > \beta_{\text{th}} = 1/\sqrt{12} \approx 0.29$, both the propagating electromagnetic waves in vacuum and surface waves at the vacuum–PTC interface can be observed, as shown in Fig. S5B. As mentioned in

S2 above, a high static permittivity $\varepsilon_r$ implicates flat dispersion curves; thereby the operating range becomes wide, as illustrated in the shaded region in Fig. S5D, allowing us to detect and identify low-energy particles when their velocity is small. Furthermore, the radiation angle reads $\theta_v = \arccos 1/(3\beta) \approx 34^\circ$ when $\beta = 0.4$, which agrees with the theoretical prediction given in the main text.

### S3.3 When $\beta_{\text{th}}$ is small

In the main text, it is given that the radiation angle $\theta_{v,n}$ for the $n$-th order propagating waves can be determined by the electron velocity $\beta c_0$ and the mode number $n$, which reads

$$\cos\theta_{v,n} = \frac{k_x}{k_{b,n}} = \frac{\omega_{b,0}/(\beta c_0)}{\omega_{b,n}/c_0} = \frac{1}{\beta}\frac{1}{2n+1}. \tag{S11}$$

Here, (S11) indicates that the allowed order $n$ of the propagating waves (harmonics) in vacuum should satisfy

$$n \geq \frac{1}{2}\left(\frac{1}{\beta} - 1\right) \tag{S12}$$

for positive integers in order to manifest $\cos\theta_v \leq 1$. Therefore, low-order propagating modes in vacuum may be absent when the velocity of particles is small according to (S12). When the static permittivity reads $\varepsilon_r > (2n+1)^2$ with the corresponding threshold $\beta_{\text{th}} < (2n+1)^{-1}$, the lowest order of the propagation mode in vacuum is $n_p = n+1$ for $\beta_{\text{th}} < \beta < (2n+1)^{-1}$. For example, when considering a PTC with a static permittivity of $\varepsilon_r = 12 > (2n+1)^2$ for $n = 1$, particles with different velocities generate modes with different lowest order $n_p$, as illustrated in Fig. S6A and Fig. S6B. When the particle velocity $\beta = 0.6 > (2n+1)^{-1} = 1/3$ for $n = 1$, the primary propagating mode can be observed in vacuum, the radiation angle of which is $\theta_{v,1} = 56^\circ$, as shown in Fig. S6A. This radiation angle $\theta_{v,1}$ agrees with the angle calculated from (S12) when $n = 1$, *i.e.*, $\cos\theta_{v,1} = 1/(3\beta)$, implicating that lowest mode order is $n_p = 1$. When the particle with velocity $\beta = 0.3 > \beta_{\text{th}} \approx 0.29$ and $\beta < (2n+1)^{-1} = 1/3$ for $n = 1$, a dominant propagating mode can also be observed, as shown in Fig. S6B, and the corresponding radiation angle reads $\theta_{v,2} = 48^\circ$. This radiation angle $\theta_{v,2}$ agrees with the angle calculated from (S12) when $n = 2$, *i.e.*, $\cos\theta_{v,2} = 1/(5\beta)$, implying that the propagating mode has the lowest order $n_p = 2$.

Fig. S6C illustrates the band structure for PTCs corresponding to Fig. S6A and Fig. S6B. When the velocity of particles $\beta = 0.6 > (2n+1)^{-1} = 1/3$ for $n = 1$, the confined mode with frequency $\omega_{b,0}$ and corresponding tangential momentum $k_{e,p}$ (see Fig. S6A) can be converted into propagating modes in vacuum, with frequencies $\omega_{b,n\geq 1}$ and corresponding wave numbers $k_{b,n\geq 1}$, as indicated by the green trajectories with arrows in Fig. S6C. Likewise, when the velocity of particles $\beta = 0.3 > \beta_{\text{th}}$ and $\beta < (2n+1)^{-1} = 1/3$ for $n = 1$, for the confined mode with frequency $\omega_{b,0}$ and tangential wave vector $k_{e,q}$ (see Fig. S6B), the first order harmonic behaves

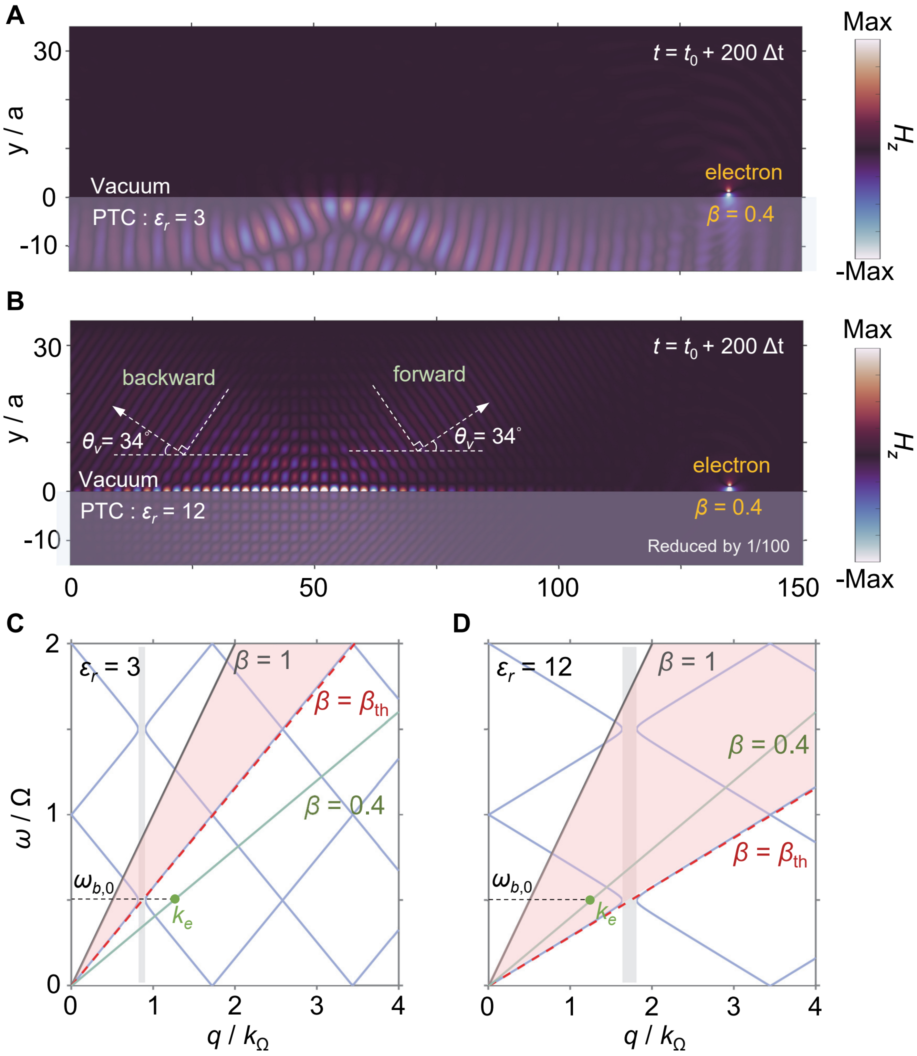


Figure S5: **Light emissions when the velocity of particles is below and above the threshold.** (**A** and **B**) Near-field magnetic field $H_z$ distribution for a electron travelling in close proximity of the PTC, whose velocity $\beta = 0.4$ is below and above the threshold $\beta_{\text{th}}$, respectively, when $t = t_0 + 200\,\Delta t$. The modulation function of the PTC reads $\varepsilon_{\text{sin}}(t) = \varepsilon_r(1 + \alpha\ \sin\Omega t)$ with the modulation depth $\alpha = 0.2$ and the modulation frequency $\Omega = 0.2\ \omega_0$. The static permittivity is $\varepsilon_r = 3$ and $\varepsilon_r = 12$, respectively. (**C** and **D**) Band structures for PTCs when the static permittivity is $\varepsilon_r = 3$ and $\varepsilon_r = 12$, respectively. The dispersion curves of the PTC are depicted in blue; the black line represents the light line in vacuum when $\beta = 1$; the green line represents the dispersion relationship of confined wave near the electron with velocity $\beta = 0.4$; the red dashed line represents the threshold $\beta = \beta_{\text{th}} = 1/\sqrt{\varepsilon_r}$ in the PTC. Red-shaded regions illustrate the range for which confined modes can be converted into propagating modes.

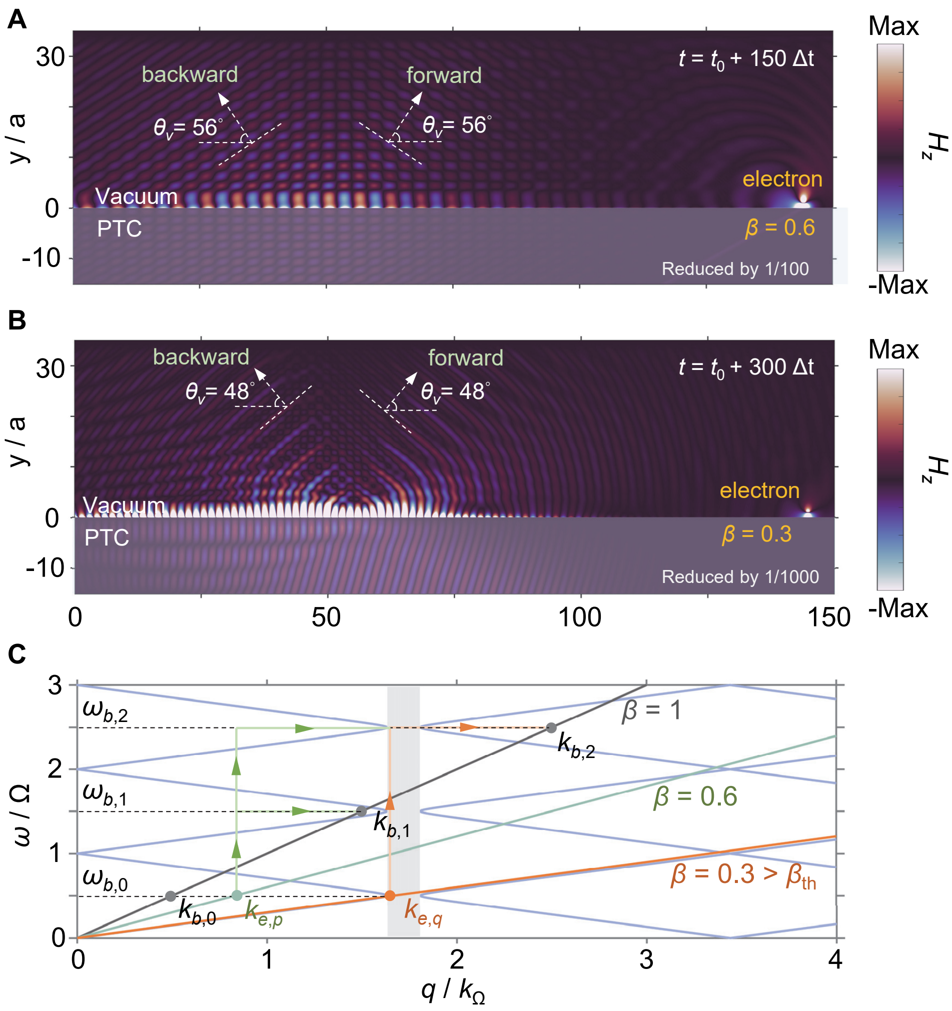


Figure S6: **Light emission when the static permittivity $\varepsilon_r$ is large.** The modulation function of the PTC reads $\varepsilon_{\sin}(t) = \varepsilon_r(1+\alpha \sin\Omega t)$, where the static permittivity $\varepsilon_r = 12$, the modulation depth and frequency are $\alpha = 0.2$ and $\Omega = 0.2\ \omega_0$, respectively. (**A** and **B**) Near-field magnetic field distribution $H_z$ for electrons traveling in close proximity over the PTC, for which the velocity of the electron reads $\beta = 0.6$ and $\beta = 0.3$, respectively. The field profiles correspond to the time steps when $t = t_0 + 150\ \Delta t$ and $t = t_0 + 300\ \Delta t$, respectively, where $t_0$- denotes the start time of the modulation and $\Delta t$ denotes the time step in the simulation. (**C**) Band structure of the PTC. The dispersion curves of the PTC are colored blue. The black line represents the light line as a reference; the orange and green lines represent the dispersion relationship of confined waves near the electron with velocity $\beta = 0.3$ and $\beta = 0.6$, respectively. The paths of mode evolution, characterized by velocity $\beta = 0.3$ and $\beta = 0.6$, are illustrated by orange and green lines with arrows, respectively.

as a surface wave restricted at the vacuum–PTC interface, and only the high order harmonics can propagate in vacuum, with radiated frequencies $\omega_{b,n\geq 2}$ and corresponding wave numbers $k_{b,n\geq 2}$, as indicated by the orange trajectories with arrows in Fig. S6C. Thus, for a particle with velocity $\beta > \beta_{\rm th}$, the lowest order of the propagating mode in vacuum can be determined by $n_p = \lceil (1/\beta - 1)/2 \rceil$. In addition, higher modes for $n > n_p$ would be weak and negligible; as a result, highly directional propagating waves of frequency $\omega_{b,n} = (n_p + 1/2)\Omega$ may be detected, whose radiation angle is determined by (S11) where $n = n_p$.

## S4 Details of finite-difference time-domain simulations

The Python interface of the open source software package MEEP was used, which is based on the finite difference time domain (FDTD) method (*11*). In the simulation, the scale-invariant units are adopted and the simulation parameters are: $\omega_0 = 2\pi$, characteristic length $a = 1$; space resolution $N_{\rm resolution} = 20$; time step $\Delta t = 0.025$. In MEEP, the spatial distribution and time characteristics of the Gaussian beam can be set by the `GaussianBeamSource` class and the `GaussianSource` subclass, respectively, which were used to illustrate the interaction of plane waves with the PTC in **Figure 1** of the main text. As for moving charged particles, they can be mimiced by the electric-charge current with a small geometric scale, whose center position can be specified by the built-in function `change_sources`. The current source is $x$-polarized and its velocity reads $\beta c_0 \hat{\mathbf{x}}$. Theoretically, the static dipoles are adopted; however, an oscillation frequency is required in the MEEP simulation and we chose $f = 10^{-8}$, which is almost static. Interested readers can refer to the MEEP documentation for detailed code when modeling a moving-point charge. The time-varying PTC is simulated by updating the permittivity of the medium at each time step using the built-in function `change_materials`. The entire simulation domain is truncated by perfectly matched layers (PMLs). In the post-processing visualization of **Figure 2** in the main text, to emphasize the contour of the radiated plane waves, the radiated field during time modulation was subtracted by the corresponding radiation field without time modulation.

# References and Notes


1. J. Donohue, J. Gardelle, *Phys. Rev. ST Accel. Beams* **8**, 060702 (2005).

2. D. Li, Z. Yang, K. Imasaki, G.-S. Park, *Phys. Rev. ST Accel. Beams* **9**, 040701 (2006).

3. H. L. Andrews, C. H. Boulware, C. A. Brau, J. D. Jarvis, *Phys. Rev. ST Accel. Beams* **8**, 050703 (2005).

4. H. Andrews, C. Brau, *Phys. Rev. ST Accel. Beams* **7**, 070701 (2004).

5. D. Li, *et al.*, *Free electron lasers*, S. Varro, ed. (IntechOpen, Rijeka, 2012), chap. 6.

6. H. L. Andrews, C. H. Boulware, C. A. Brau, J. D. Jarvis, *Phys. Rev. ST Accel. Beams* **8**, 110702 (2005).
7. W. Liu, Z. Xu, *New J. Phys.* **16**, 073006 (2014).
8. P. Zhang, Y. Zhang, M. Tang, *Opt. Express* **25**, 10901 (2017).
9. I. M. Frank, I. Tamm, *Dokl. Akad. Nauk SSSR* **14**, 109 (1937).
10. S. J. Smith, E. M. Purcell, *Phys. Rev.* **92**, 1069 (1953).
11. A. F. Oskooi, *et al.*, *Comput. Phys. Commun.* **181**, 687 (2010).


Dated: November 2, 2023
